# Supplementary material for: Distributional Transform Based Information Reconciliation
Source: arXiv:2204.08891 source file (2023-05-11)
Supplement: Supplementary file 1 [file appendix.tex]

\section{Copula Theory in a Nutshell}
